# Supplementary material for: Contact-Aware Non-prehensile Robotic Manipulation for Object Retrieval in Cluttered Environments
Source: arXiv:2303.03635 source file (2023-03-07)
Supplement: Supplementary file 1 [file 7_appendix.tex]

In appendix, we provide the proof of Prop.~\ref{thm: value iteration convergence}.
For simplicity, we only give the proof for $V^{\pi_{dy}}$.
The statement of $Q^{\pi_{dy}}$ can be derived similarly.
Denote the state sequence $(s_1, \cdots, s_n)$ as $s_{1:n}$, and further define the operator $T$ as:
\vspace{-5pt}
\begin{equation}
    \begin{split}
    Tx = &\mathbb{E}_{(a, n)\sim \pi_{dy}(\cdot|s_0)}
    \Big[ \mathbb{E}_{(s_1, s_2, \cdots, s_n) \sim P_{dy}(\cdot|s_0, a, n)} \Big[\\
    & \sum_{t=0}^{n-1} \gamma^t r(s_t, a, s_{t+1}) + \gamma^n x \Big]\Big].
    \end{split}
    \vspace{-5pt}
\end{equation}

To prove the proposition, we only need to show that the operator $T$ is a contraction mapping, and then we can derive the proposition by the Banach fixed-point theorem.

Let $d(x, y) = || x-y ||_\infty$, then we have
% \vspace{-5pt}
\begin{equation}
\begin{split}
        & d(Tx, Ty) = \Big\| Tx - Ty \Big\|_\infty\\
         &= \Big\| \mathbb{E}_{(a, n)\sim \pi_{dy}(\cdot|s_0)}
    \Big[ \mathbb{E}_{s_{1:n} \sim P_{dy}(\cdot|s_0, a, n)} \big[\gamma^n (x-y) \big] \Big] \Big\|_\infty\\
    & = \Big\| \sum_{a, n} \gamma^n \pi_{dy}(a, n | s_0) \sum_{s_{1:n}} P_{dy}(s_{1:n} | s_0, a, n) (x-y) \Big\|_\infty \\
    & \le \Big\| \sum_{a, n} \gamma^n \pi_{dy}(a, n | s_0) \sum_{s_{1:n}} P_{dy}(s_{1:n} | s_0, a, n) \Big\|_\infty \cdot \Big\| x-y \Big\|_\infty \\
    & = \Big\| \sum_{a, n} \gamma^n \pi_{dy}(a, n | s_0) \Big\|_\infty \cdot \Big\| x-y \Big\|_\infty. \nonumber
\end{split}
\end{equation}
Notice that $\sum_{a, n} \pi_{dy}(a, n | s_0) = 1$, $\pi_{dy}(\cdot|s_0) \ge 0$, and $\gamma \in [0, 1)$.
Therefore, $\left\| \sum_{a, n} \gamma^n \pi_{dy}(a, n | s_0) \right\|_\infty \in [0, 1)$.
Denoting $K = \left\| \sum_{a, n} \gamma^n \pi_{dy}(a, n | s_0) \right\|_\infty$,
then $d(Tx, Ty) \le K d(x, y)$.
Hence $T$ is a contraction mapping. \hfill $\square$
